# Supplementary material for: Polynomial Precision Dependence Solutions to Alignment Research Center Matrix Completion Problems
Source: arXiv:2401.03999 source file (2024-01-08)
Supplement: Supplementary file 1 [file appendix.tex]

\appendix

\section{Solving Iteration Subproblems}
\label{sec:ipm}
In this section, we detail the primal-dual path-following interior point methods used to solve the small semidefinite program to compute the value $\hat{f}_t(\tilde{y}_{t+1})$ and the small quadratic semidefinite program~\eqref{eq:small_quad_sdp}.
Before we can derive the algorithms, it is necessary to define the $\svec$ operator and symmetric Kronecker product~\cite{alizadeh1998primal,schacke2004kronecker,todd1998nesterov}.

For any matrix $A \in \SS^n$, the vector $\svec(A) \in \RR \mathclose{\vphantom{\big)}}^{n+1 \choose 2}$ is defined as
\begin{equation*}
\svec(A) = \left[ a_{11}, \sqrt{2} a_{21}, \ldots, \sqrt{2} a_{n1}, a_{22}, \sqrt{2} a_{32}, \ldots, \sqrt{2} a_{n2}, \ldots, a_{nn}\right]^\top.
\end{equation*}
The $\svec$-operator is a structure preserving map between $\SS^n$ and $\RR\mathclose{\vphantom{\big)}}^{n+1 \choose 2}$ where the constant $\sqrt{2}$ multiplied by some of the entries ensures that
\begin{equation*}
\langle A, B \rangle = \tr(AB) = \svec(A)^\top \svec(B), \quad \forall\, A, B \in \SS^n.
\end{equation*}
For any $M \in \RR \mathclose{\vphantom{)}}^{n \times n}$, let $\textrm{vec}(M)$ be the map from $\RR \mathclose{\vphantom{)}}^{n \times n}$ to $\RR \mathclose{\vphantom{)}}^{n^2}$ defined by stacking the columns of $M$ into a single $n^2$-dimensional vector.
It is also useful to define the matrix $ U \in \RR\mathclose{\vphantom{\big)}}^{{n+1 \choose 2} \times n^2}$ which maps $\textrm{vec}(A) \mapsto \svec(A)$ for any $A \in \SS^n$. Let $u_{ij,kl}$ be the entry in the row which defines element $a_{ij}$ in $\svec(A)$ and the column that is multiplied with the element $a_{kl}$ in $\textrm{vec}(A)$.
Then
\begin{equation*}
    u_{ij,kl} = \begin{cases}
        1 & \quad i = j = k = l \\
        \frac{1}{\sqrt{2}} & \quad i = k\ne j = l \textrm{, or } i = l \ne j = k \\
        0 & \quad \textrm{o.w.}
    \end{cases}
\end{equation*}
As an example, the case when $n=2$:
\begin{equation*}
  U = \begin{bmatrix}
      1 & 0& 0& 0 \\
      0 & \frac{1}{\sqrt{2}}& \frac{1}{\sqrt{2}} & 0 \\
      0 & 0& 0& 1 \\
  \end{bmatrix}.  
\end{equation*}
Note that $U$ is a unique matrix with orthonormal rows and has the following property
\begin{equation*}
    U^\top U \textrm{vec}(A) = U^\top \svec(A) = \textrm{vec}(A), \quad \forall \, A \in \SS^n.
\end{equation*}

The symmetric Kronecker product $\otimes_s$ can be defined for any two square matrices $G, H \in \RR^{n\times n}$ by its action on a vector $\svec(A)$ for $A \in \SS^n$ as follows
\begin{equation*}
(G \otimes_s H)\, \svec(A) = \frac{1}{2} \svec(HAG^\top + GAH^\top).
\end{equation*}
Alternatively, but equivalently~\cite{schacke2004kronecker}, the symmetric Kronecker product can be defined more explicitly using the matrix $U$ defined above as follows
\begin{equation*}
G \otimes_s H = \frac{1}{2} U( G \otimes H + H \otimes G) U^\top,
\end{equation*}
where $\otimes$ is the standard Kronecker product. We use this latter definition in our implementation.

\subsection{Computing $\hat{f}_t(\tilde{y}_{t+1})$}
\label{sec:ipm_lb_spec_est}
The value $\hat{f}_t(\tilde{y}_{t+1})$ is the optimum value of the following optimization problem (remember that $\nu$ can be dropped since $\tilde{y}_{t+1}$ is always feasible)
\begin{equation*}
\begin{aligned}
&\maximize \quad \langle C - \cA\adj \tilde{y}_{t+1}, \eta \bar{X}_t + V_t S V_t^\top \rangle + \langle b, \tilde{y}_{t+1}\rangle\\
&\st \;\;\; \eta \geq 0 \\
&\qquad\qquad\quad\;\; S \succeq 0 \\
&\qquad\qquad\quad\;\; \eta + \tr(S) \leq \alpha
\end{aligned}
\end{equation*}
This amounts to computing $\langle C - \cA\adj \tilde{y}_{t+1}, \eta_\star \bar{X}_t + V_t S_\star V_t^\top \rangle + \langle b, \tilde{y}_{t+1}\rangle$ where $(\eta_\star, S_\star)$ is a solution to the following (small) semidefinite program
\begin{equation}
\label{eq:compressed_subprob_1}
\begin{aligned}
&\minimize \quad g_1^\top \svec(S) + \eta \, g_2\\
&\st \;\;\; \eta \geq 0 \\
&\qquad\qquad\quad\;\; S \succeq 0 \\
&\qquad\qquad\quad\;\; 1 - v_I^\top \svec(S) - \eta \geq 0
\end{aligned}
\end{equation}
where 
\begin{equation*}
    \begin{aligned}
        g_1 &= \alpha \,\svec(V_t^\top\!(\cA\adj\tilde{y}_{t+1} - C) V_t), \\
        g_2 &= \frac{\alpha}{\tr\!\left(\bar{X}\right)} \langle \bar{X}_t, \cA\adj\tilde{y}_{t+1} - C) \rangle, \\
        v_I &= \svec(I).  \qquad (I \textrm{ is the } k \times k \textrm{ identity matrix})
    \end{aligned}
\end{equation*}

We will use a primal-dual interior point method to solve~\eqref{eq:compressed_subprob_1}.
We follow the well known technique for deriving primal-dual interior point methods~\cite{helmberg1994interior}. 
We start by defining the Lagrangian of the dual barrier problem of~\eqref{eq:compressed_subprob_1},
\begin{equation}
\label{eq:dual_barrier_Lagrangian1}
\begin{aligned}
L_\mu(S, \eta, T, \zeta, \omega) &= g_1^\top \svec(S) + \eta g_2 - \svec(S)^\top\svec(T) - \eta \zeta \\
&\qquad- \omega(1 - v_I^\top \svec(S) - \eta) + \mu (\log \det (T) + \log\zeta + \log \omega),
\end{aligned}
\end{equation}
where we introduce a dual slack matrix $T \succeq 0$ as complementary to $S$, a dual slack scalar $\zeta \geq 0$ as complementary to $\eta$, a Lagrange multiplier $\omega \geq 0$ for the trace constraint inequality, and a barrier parameter $\mu > 0$.
Notice that we have moved from needing to optimize a constrained optimization problem to an unconstrained optimization problem.
The saddle point solution of~\eqref{eq:dual_barrier_Lagrangian1} is given by the solution of the KKT-conditions, which reduces to just the first-order optimality conditions since the problem is unconstrained.
The first-order optimality conditions of~\eqref{eq:dual_barrier_Lagrangian1} are the following system of equations
\begin{align}
\nabla_S L_\mu &= g_1 - \svec(T) + \omega v_I = 0 \label{eq:kkt_1}\\
\nabla_\eta L_\mu &= g_2 - \zeta + \omega = 0 \label{eq:kkt_2}\\
\nabla_T L_\mu &= S - \mu T^{-1} = 0 \label{eq:kkt_3}\\
\nabla_\zeta L_\mu &= \eta - \mu \zeta^{-1} = 0 \label{eq:kkt_4}\\
\nabla_\omega L_\mu &= 1 - v_I^\top \svec(S) - \eta - \mu \omega^{-1} = 0 \label{eq:kkt_5}
\end{align}
By the strict concavity of $\log \det T$, $\log \zeta$, and $\log \omega$, there exists a unique solution $(S_\mu, \eta_\mu, T_\mu, \zeta_\mu, \omega_\mu)$ to this system of equations for any value of the barrier parameter $\mu > 0$.
The sequence of these solutions as $\mu \to 0$ forms the \emph{central trajectory} (also known as the central \emph{path}).
For a point $(S, \eta, T, \zeta, \omega)$ on the central trajectory, we can use any combination of~\eqref{eq:kkt_3},~\eqref{eq:kkt_4}, and/or~\eqref{eq:kkt_5} to solve for $\mu$,
\begin{equation}
    \label{eq:barrier_param_est}
    \mu = \frac{\langle S, T \rangle}{k} = \eta \zeta = \omega(1 - v_I^\top \svec(S) - \eta) = \frac{\langle S, T \rangle + \eta \zeta + \omega(1 - v_I^\top \svec(S) - \eta)}{k + 2}.
\end{equation}

The fundamental idea of primal-dual interior point methods is to use Newton's method to follow the central path to a solution of~\eqref{eq:compressed_subprob_1}.
Before we can apply Newton's method, we must linearize the non-linear equations ~\eqref{eq:kkt_3},~\eqref{eq:kkt_4}, and~\eqref{eq:kkt_5} into an equivalent linear formulation.
There are several ways one could linearize these equations and the choice of linearization significantly impacts the algorithm's behavior (see~\cite{alizadeh1998primal} or~\cite{helmberg1994interior} for more on the choice of linearization).
We choose one standard method linearization, detailed in the following system
of equations
\begin{equation}
    \label{eq:linearized_system1}
    \mathrm{F}_\mu(\theta) = \mathrm{F}_\mu(S, \eta, T, \zeta, \omega) := \begin{pmatrix}
        \vspace{0.1em} g_1 - \svec(T) + \omega v_I \\
        \vspace{0.1em} g_2 - \zeta + \omega \\
        \vspace{0.1em} ST - \mu I \\
        \vspace{0.1em} \eta\zeta - \mu\\
        \vspace{0.1em} \omega (1 - v_I^\top \svec(S) - \eta) - \mu\\
    \end{pmatrix}
    = 0.
\end{equation}
The solution $\theta_\star$ to this system of equations $\mathrm{F}_\mu(\theta) = 0$ satisfies the first-order optimality conditions~\eqref{eq:kkt_1}-\eqref{eq:kkt_5} and is the optimal solution to the barrier problem.
We utilize Newton's method to take steps in the update direction $\Delta \theta = (\Delta S, \Delta \eta, \Delta T, \Delta \zeta, \Delta \omega)$ towards $\theta_\star$.
The update direction $\Delta \theta$ determined by Newton's method must satisfy the following equation
\begin{equation*}
    \mathrm{F}_\mu(\theta) + \nabla \mathrm{F}_\mu(\Delta \theta) = 0.
\end{equation*}
Hence, the update direction $\Delta \theta$ is the solution to the following system of equations (after the same standard linearization has been applied to the following system as in~\eqref{eq:linearized_system1})
\begin{align}
- \svec(\Delta T) + \Delta \omega \, v_I &= \svec(T) - g_1 - \omega \, v_I \\
- \Delta \zeta + \Delta \omega &= \zeta - g_2 - \omega \\
\omega^{-1}(1 - v_I^\top \svec(S) - \eta) \Delta \omega - v_I^\top \svec(\Delta S) - \Delta \eta &= \mu \omega^{-1} + v_I^\top \svec(S) + \eta - 1 \\
(T \otimes_s S^{-1}) \, \svec(\Delta S) + \svec(\Delta T) &= \mu \,\svec(S^{-1}) - \svec(T) \\
\zeta \eta^{-1} \Delta \eta + \Delta \zeta &= \mu \eta^{-1} - \zeta
\end{align}
We can solve this system efficiently by analytically eliminating all variables except $\svec(\Delta S)$. We can compute $\svec(\Delta S)$ by solving the following linear matrix equation using an off-the-shelf linear system solver
\begin{equation}
\label{eq:delta_S_linear_system}
\begin{aligned}
&\left( T \otimes_s S^{-1} + \frac{\zeta \eta^{-1}}{\kappa_1 \zeta \eta^{-1} + 1} v_I v_I^\top \right) \svec(\Delta S) 
= v_I g_2 - v_I \mu \eta^{-1} - g_1 + \mu \, \svec(S^{-1}) \\
&\qquad\qquad + v_I \zeta \eta^{-1} (- \kappa_1 \zeta \eta^{-1} - 1)^{-1} \left(-\kappa_1 (\mu \eta^{-1} - g_2 - \omega) + \mu \omega^{-1} + v_I^\top \svec(S) + \eta - 1\right)
\end{aligned}
\end{equation}
where $\kappa_1 := \omega^{-1}(1 - v_I^\top \svec(S) - \eta)$.
Then, computing the rest of the update directions $\Delta \eta$, $\svec(\Delta T)$, $\Delta \zeta$, and $\Delta \omega$ amounts to back-substituting the solution to~\eqref{eq:delta_S_linear_system} for $\svec(\Delta S)$ through the analytical variable elimination equations.

Given how to compute the update directions, the primal-dual interior point method proceeds as follows. Initialize the variables $\theta = (S, \eta, T, \zeta, \omega)$ to an arbitrary strictly feasible point (i.e. $S \succ 0$, $\eta > 0$, $T \succ 0$, $\zeta > 0$, and $\omega > 0$). Starting from this primal-dual pair we compute an estimate of the barrier parameter as follows
\begin{equation*}
    \mu \gets \frac{\langle S, T \rangle + \eta \zeta + \omega (1 - v_I^\top \svec(S) - \eta)}{2(k + 2)},
\end{equation*}
where, as done in~\cite{helmberg1994interior}, we use~\eqref{eq:barrier_param_est} and divide by two.
Then, we compute the update direction $\Delta \theta$ as described above and perform a backtracking line search to find a step size $\delta \in (0, 1]$ such that $\theta + \delta \, \Delta \theta$ is again strictly feasible.
Lastly, following~\cite{helmberg2000spectral}, we compute a non-increasing estimate of the barrier parameter 
\begin{equation*}
    \mu \gets \min \left\{ \mu_\textrm{prev}, \gamma \frac{\langle S, T \rangle + \eta \zeta + \omega (1 - v_I^\top \svec(S) - \eta)}{2(k + 2)}\right \}
    \quad \textrm{where} \quad 
    \gamma = \begin{cases}
    1 &  \textrm{if }\delta \leq \frac{1}{5} \\
    \frac{5}{10} - \frac{4}{10} \delta^2 & \textrm{if } \delta > \frac{1}{5}
    \end{cases}.
\end{equation*}
We iterate over these steps until the barrier parameter $\mu$ is small enough (e.g. $\mu < 10^{-7}$).

\subsection{Solving~\eqref{eq:small_quad_sdp}}
\label{sec:small_quad_sdp_ipm}
The subproblem~\eqref{eq:small_quad_sdp} can be rewritten as the following (small) quadratic semidefinite program
\begin{equation*}
\begin{aligned}
&\maximize \quad \langle C - \cA\adj y_t, \eta \bar{X}_t + V_t S V_t^\top \rangle + \langle b - \tilde{\nu}, y_t \rangle - \frac{1}{2\rho} \left\| b - \tilde{\nu} - \cA (\eta \bar{X}_t + V_t S V_t^\top)\right\|_2^2\\
&\st \;\;\; \eta \geq 0 \\
&\qquad\qquad\quad\;\; S \succeq 0 \\
&\qquad\qquad\quad\;\; \eta + \tr(S) \leq \alpha
\end{aligned}
\end{equation*}
For this subproblem, unlike the subproblem solved in~\autoref{sec:ipm_lb_spec_est}, we are solving for $\eta$ and $S$ to compute the candidate iterate $\tilde{y}_{t+1}$, update the primal variable, and  update the model.
This (small) quadratic semidefinite program is equivalent to the following optimization problem

\begin{equation}
\label{eq:compressed_subprob_2}
\begin{aligned}
&\minimize \quad \frac{1}{2} \,\svec(S)^\top Q_{11} \,\svec(S) + \eta \, q_{12}^\top \, \svec(S) + \frac{1}{2} \eta^2 q_{22} + h_1^\top \svec(S) + \eta \, h_2\\
&\st \;\;\; \eta \geq 0 \\
&\qquad\qquad\quad\;\; S \succeq 0 \\
&\qquad\qquad\quad\;\; 1 - v_I^\top \svec(S) - \eta \geq 0
\end{aligned}
\end{equation}
where 
\begin{equation*}
    \begin{aligned}
        Q_{11} &= \frac{\alpha^2}{\rho} \sum_{i=1}^m \svec(V_t^\top\! A_i V_t) \,\svec(V_t^\top\! A_i V_t)^\top \\
        q_{12} &= \frac{\alpha^2}{\rho \, \tr\!\left(\bar{X}_t\right)} \,\svec\left(V_t^\top\! \cA^{*}\cA\,\bar{X}_t V_t\right) \\
        q_{22} &= \frac{\alpha^2}{\rho \, \tr\!\left(\bar{X}_t\right)^2} \left\langle \cA\bar{X}_t,\cA\bar{X}_t\right\rangle \\
        h_1 &= \alpha \,\, \svec\left(V_t^\top \!\left(\cA\adj y_t - C - \frac{1}{\rho} \cA\adj (b - \tilde{\nu}) \right) V_t\right) \\
        h_2 &= \frac{\alpha}{\tr\!\left(\bar{X}_t\right)} \left\langle \bar{X}, \, \cA\adj y_t - C - \frac{1}{\rho} \cA\adj (b - \tilde{\nu}) \right\rangle \\
        v_I &= \svec(I) 
    \end{aligned}
\end{equation*}

We follow the same derivation procedure as in~\autoref{sec:ipm_lb_spec_est}, so we proceed by including the details which differ from the previous section.
The Lagrangian of the dual barrier problem of~\eqref{eq:compressed_subprob_2} is as follows
\begin{equation}
\label{eq:dual_barrier_Lagrangian2}
\begin{aligned}
L_\mu(S, \eta, T, \zeta, \omega) &= \frac{1}{2} \,\svec(S)^\top Q_{11} \,\svec(S) + \eta \, q_{12}^\top \, \svec(S) \\ &\qquad+ \frac{1}{2} \eta^2 q_{22} + h_1^\top \svec(S) + \eta \, h_2 - \svec(S)^\top\svec(T) - \eta \zeta \\
&\qquad- \omega(1 - v_I^\top \svec(S) - \eta) + \mu (\log \det (T) + \log\zeta + \log \omega).
\end{aligned}
\end{equation}
The first-order optimality conditions of~\eqref{eq:dual_barrier_Lagrangian2} yields the following system of equations (after the same standard linearization)
\begin{equation}
    \label{eq:linearized_system2}
    \mathrm{F}_\mu(S, \eta, T, \zeta, \omega) := \begin{pmatrix}
        \vspace{0.1em} Q_{11}\, \svec(S) + \eta \,q_{12} + h_1 - \svec(T) + \omega v_I \\
        \vspace{0.1em} q_{12}^\top \, \svec(S) + \eta \,q_{22} + h_2 - \zeta + \omega \\
        \vspace{0.1em} ST - \mu I \\
        \vspace{0.1em} \eta\zeta - \mu\\
        \vspace{0.1em} \omega (1 - v_I^\top \svec(S) - \eta) - \mu\\
    \end{pmatrix}
    =: \begin{pmatrix}
        \vspace{0.1em} \mathsf{F}_1 \\
        \vspace{0.1em} \mathsf{F}_2 \\
        \vspace{0.1em} \mathsf{F}_3 \\
        \vspace{0.1em} \mathsf{F}_4 \\
        \vspace{0.1em} \mathsf{F}_5 \\
    \end{pmatrix}
    = 0.
\end{equation}
The Newton's method step direction $(\Delta S, \Delta \eta, \Delta T, \Delta \zeta, \Delta \omega)$ is determined via the following linearized system
\begin{align}
Q_{11} \svec(\Delta S) + \Delta \eta \,q_{12} - \svec(\Delta T) + \Delta \omega \, v_I &= - \mathsf{F}_1 \\
q_{12}^\top \, \svec(\Delta S) + \Delta \,\eta q_{22} - \Delta \zeta + \Delta \omega &= - \mathsf{F}_2 \\
\omega^{-1}(1 - v_I^\top \svec(S) - \eta) \Delta \omega - v_I^\top \svec(\Delta S) - \Delta \eta &= \mu \omega^{-1} + v_I^\top \svec(S) + \eta - 1 \\
(T \otimes_s S^{-1}) \, \svec(\Delta S) + \svec(\Delta T) &= \mu \,\svec(S^{-1}) - \svec(T) \\
\zeta \eta^{-1} \Delta \eta + \Delta \zeta &= \mu \eta^{-1} - \zeta
\end{align}
We can solve this system efficiently by analytically eliminating all variables except $\svec(\Delta S)$. We can compute $\svec(\Delta S)$ by solving the following linear matrix equation using an off-the-shelf linear system solver
\begin{equation}
\label{eq:delta_S_linear_system2}
\begin{aligned}
&\left( Q_{11} + T \otimes_s S^{-1} - (\kappa_1 \kappa_2 + 1)^{-1}\big( q_{12} (\kappa_1 q_{12} + v_I)^\top \!+ v_I(q_{12} - \kappa_2 v_I)^\top\big)\right)  \svec(\Delta S) \\
&\qquad=  q_{12} \left( (\kappa_1 \kappa_2 + 1)^{-1}\left( \mu \omega^{-1} + v_I^\top \svec(S) + \eta - 1 + \kappa_1 (\textsf{F}_2 - \mu \eta^{-1} + \zeta)\right)\right) \\
&\qquad\qquad + v_I\left((\kappa_1 \kappa_2 + 1)^{-1} \left( \textsf{F}_2 - \mu \eta^{-1} + \zeta - \kappa_2 (\mu \omega^{-1} + v_I^\top \svec(S) + \eta - 1) \right)\right) \\
&\qquad\qquad-\textsf{F}_1 + \mu \,\svec(S^{-1}) - \svec(T),
\end{aligned}
\end{equation}
where $\kappa_1 := \omega^{-1}(1 - v_I^\top \svec(S) - \eta)$ and $\kappa_2 := \zeta \eta^{-1} + q_{22}$.
Then, computing the rest of the update directions $\Delta \eta$, $\svec(\Delta T)$, $\Delta \zeta$, and $\Delta \omega$ amounts to back-substituting the solution to~\eqref{eq:delta_S_linear_system2} for $\svec(\Delta S)$ through the analytical variable elimination equations.

We make a single change to the initialization as compared with the interior point method presented in~\autoref{sec:ipm_lb_spec_est}. Since this interior point method can be executed multiple times in a row with only the value of $\tilde{\nu}$ changing as the first step in the alternating maximization algorithm, we warm-start initialize $\theta$ with the previous execution's $\theta_\star$. We observe non-negligible convergence improvements over arbitrary initialization as this interior point method procedure is called in sequence.

\section{Proofs of Theoretical Results}

\subsection{Proof of Fact~\ref{fact:bounded}}
\label{sec:bounded_proof}
The function $f$ is continuous and proper over the domain $\cY$.
It is a well-known fact that the level sets of continuous proper functions are compact. 
Hence, the union of level sets $\{y \in \cY : f(y_\star) \leq f(y) \leq f(y_0)\}$ is compact, and therefore, $\sup_{\,t \geq 0} \{\dist(y_t, \cY_*)\} < \infty$.
The subgradients take the form $g_{t+1} = b + \alpha \cA(v v^{\!\top}) \in \partial f(\tilde{y}_{t+1})$ where $v \in \RR^n$ is a unit-normed vector, and thus, $\|g_{t+1}\| < \infty$ for all $t$. 

\subsection{Proof of Lemma~\ref{lem:error_bound}}
\label{sec:error_bound_proof}
Let $\cF := \{y \in \RR^m : \cA\adj y - C \in \SS^n_+\}$. Observe that $\cY_\star = \cY \cap \cF$.
Since $\cY_\star$ is compact, the H\"olderian error bound~\cite{sturm2000error, drusvyatskiy2017many, sremac2021error} ensures that
\begin{equation*}
\dist(y, \cY_\star) \leq \cO \left(\dist^{2^{-d}}(y, \cY) + \dist^{2^{-d}}(y, \cF)\right),
\end{equation*}
where $d \in \{0, 1, \ldots, m\}$ is the singularity degree of the SDP.
This implies that for $y \in Y$,
\begin{equation*}
\begin{aligned}
\dist^{2^{d}}(y, \cY_\star) &\leq \cO \left(\dist(y, \cF)\right) \\
&\leq \cO \left( \alpha \max \{ \lambda_\textrm{max}(C - \cA\adj y), 0\} \right) \\
&\leq \cO \left( f(y) - f(y_\star) \right).
\end{aligned}
\end{equation*}

\subsection{Proof of Lemma~\ref{lem:primal_feasibility}}
\label{sec:primal_feasibility_proof}
For any descent step $t$, it is easy to verify from~\ref{eq:dual_update} and~\eqref{eq:dual_slack_update} that 
\begin{equation*}
    \proj_\cK(\cA X_{t+1}) - \cA X_{t+1} \leq \rho (y_t - y_{t+1}),
\end{equation*}
and therefore,
\begin{equation*}
    \| \cA X_{t+1} -  \proj_\cK(\cA X_{t+1})\|^2 \leq \rho^2 \| y_t - y_{t+1} \|^2.
\end{equation*}
To complete the proof we utilize the fact that $\hat{f}_t(y_{t+1}) = \min_{y \in \cY} \hat{f}_t(y) + \frac{\rho}{2}\|y - y_t\|^2$, the fact that $\hat{f}_t(y) \leq f(y)$ for all $y \in \cY$, and the definition of a descent step, which gives
\begin{equation*}
    \frac{\rho}{2} \|y_{t+1} - y_t\|^2 \leq \hat{f}_t(y_t) - \hat{f}_t(y_{t+1}) \leq f(y_t) - \hat{f}_t(y_{t+1}) \leq \frac{f(y_t) - f(y_{t+1})}{\beta} \leq \frac{f(y_t) - f(y_\star)}{\beta}.
\end{equation*}
Assume Slater's condition holds and $y_\star$ is unique. Then, using Lemma~\ref{lem:error_bound} gives
\begin{equation*}
\begin{aligned}
    \| \cA X_{t+1} -  \proj_\cK(\cA X_{t+1})\|^2 &\leq \rho^2 \| y_t - y_{t+1} \|^2\\
    &\leq \rho^2 \left(\|y_t - y_\star\|^2 + \|y_{t+1} - y_\star\|^2\right) \\
    &\leq \cO\!\left((f(y_t) - f(y_\star))^2\right) + \cO\!\left((f(y_{t+1}) - f(y_\star))^2\right) \\
    &\leq  \cO\!\left((f(y_t) - f(y_\star))^2\right).
\end{aligned}
\end{equation*}

\subsection{Proof of Lemma~\ref{lem:dual_feasibility}}
\label{sec:dual_feasibility_proof}
By definition of strong duality, we know that for any $X_\star \in \cX_\star$ that $\langle C, X_\star \rangle = \langle b, y_\star \rangle$, and equivalently, $\langle X_\star, \cA\adj y_\star - C \rangle = 0$.
Then, the dual objective gap is bounded as follows
\begin{align*}
\langle b, y_t - y_\star \rangle &= \langle \cA X_\star, y_t - y_\star \rangle \\
&= \langle X_\star, \cA\adj(y_t - y_\star)\rangle \\
&= \langle X_\star, (\cA\adj y_t - C) - (\cA\adj y_\star - C) \rangle \\
&= \langle X_\star, \cA\adj y_t - C \rangle \\
&\geq - \| X_\star \|\nuc \max\{\lambda_{\max}(C - \cA\adj y_t), 0\}.
\end{align*}
We now utilize this bound to obtain the desired result
\begin{equation*}
f(y_t) - f(y_\star) = \langle b, y_t - y_\star \rangle + \alpha \max\{ \lambda_{\max} (C - \cA\adj y_t), 0\} \geq \| X_\star \|\nuc \max\{ \lambda_{\max}(C - \cA\adj y_t), 0\},
\end{equation*}
where the last inequality is implied by the assumption that $\alpha \geq 2 \NN(\cX_\star) \geq 2 \|X_\star\|\nuc$.

\subsection{Proof of Lemma~\ref{lem:primal_dual_opt}}
\label{sec:primal_dual_opt_proof}
We start by rewriting the primal-dual gap as follows
\begin{align*}
    \langle C, X_{t+1} \rangle - \langle b, y_{t+1} \rangle
   &= \langle C, X_{t+1} \rangle - \langle \cA X_{t+1}, y_{t+1}\rangle  + \langle \cA X_{t+1} - b, y_{t+1} \rangle \\
   &= \langle X_{t+1}, C - \cA\adj y_{t+1}\rangle + \langle \cA X_{t+1} - b, y_{t+1} \rangle. 
\end{align*}
We will now bound the absolute values of the two resulting terms to bound the desired quantity.
Using the Cauchy-Schwarz inequality and Lemma~\ref{lem:primal_feasibility} it can be seen
\begin{align*}
    |\langle \cA X_{t+1} - b, y_{t+1} \rangle |
    &\leq \|\cA X_{t+1} - b\| \|y_{t+1}\| \\
    &\leq \cO\!\left(\|y_{t+1}\| \sqrt{f(y_t) - f(y_\star)} \right) \\
    &\leq \cO\!\left(\sqrt{f(y_t) - f(y_\star)} \right),
\end{align*}
where the last inequality comes from Fact~\ref{fact:bounded}.
Assume Slater's condition holds and $y_\star$ is unique. Then, using Lemma~\ref{lem:error_bound} gives
\begin{equation*}
    |\langle \cA X_{t+1} - b, y_{t+1} \rangle |\leq \cO\left(f(y_t) - f(y_\star) \right).
\end{equation*}
Since $X_{t+1} \succeq 0$ and $\tr(X_{t+1}) \leq \alpha$ by construction, we can use Lemma~\ref{lem:dual_feasibility} to yield
\begin{align*}
    |\langle X_{t+1}, C - \cA\adj y_{t+1} \rangle |
    &\leq \cO(\max\{C - \cA\adj y_{t+1}, 0 \}) \\
    &\leq \cO(f(y_{t+1}) - f(y_\star)) \\
    &\leq \cO(f(y_t) - f(y_\star)).
\end{align*}
The immediately yields the desired result.

\subsection{Proof of Theorem~\ref{thm:sublinear_convergence}}
\label{sec:sublinear_convergence_proof}

The overall proof strategy is to use Theorem~\ref{thm:proximal_bundle_convergence} to show that the penalized dual gap, $f(y_t) - f(y_*)$, converges at a worst case rate of $\cO(1 / \varepsilon^3)$, which improves to $\cO(1 / \varepsilon)$ if Slater's condition or strict complementarity hold.
Then, we can use Lemmas~\ref{lem:primal_feasibility}, ~\ref{lem:dual_feasibility}, and~\ref{lem:primal_dual_opt} to obtain the stated convergence of primal feasibility, dual feasibility, and primal-dual optimality.

To apply the result of Theorem~\ref{thm:proximal_bundle_convergence}, we showed  that the norms of the iterates and subgradients of $f$ are bounded (Fact~\ref{fact:bounded}), and so all we need to do is show that the model satisfies the conditions~\eqref{eq:minorant_cond},~\eqref{eq:obj_subgrad_cond}, and \eqref{eq:model_subgrad_cond}.

Let $v$ be a maximum eigenvector $C - \cA\adj \tilde{y}_{t+1}$ \thinspace if \thinspace $\lambda_{\max}(C - \cA\adj \tilde{y}_{t+1}) > 0$ and $v = 0$, otherwise.
Then denote $g_{t+1} = b + \alpha \cA(vv^\top) \in \partial f(\tilde{y}_{t+1})$ as the subgradient of $f$ corresponding $v$ at the candidate iterate $\tilde{y}_{t+1}$.
Let $s_{t+1} = \rho (y_t - \tilde{y}_{t+1}) \in \partial \hat{f}_t(\tilde{y}_{t+1})$ be the aggregate subgradient.
Recall that at iteration $t+1$ the model approximates $\cX$ by the low-dimensional spectral set
\begin{equation*}
\widehat{\cX}_{t+1} := \left\{\eta \bar{X}_{t+1} + V_{t+1} S V_{t+1}^\top :  \eta\, \tr(\bar{X}_{t+1}) + \tr(S) \leq \alpha, \eta \geq 0, S \in \SS^k_+\right\}.
\end{equation*}
and therefore the penalized dual objective and model respectively take the following forms for any $y \in \cY$,
\begin{equation}
    \label{eq:obj_and_model_feasible}
    f(y) = \sup_{X \in \cX} \langle C - \cA\adj y , X\rangle + \langle b, y \rangle \quad \textrm{and} \quad \hat{f}_{t+1}(y) = \sup_{X \in \widehat{\cX}_{t+1}} \langle C - \cA\adj y , X\rangle + \langle b, y \rangle.
\end{equation}

\paragraph{Verifying~\eqref{eq:minorant_cond}.} The condition~\eqref{eq:minorant_cond} follows immediately from~\eqref{eq:obj_and_model_feasible}, since $\widehat{\cX}_{t+1} \subseteq \cX$.

\paragraph{Verifying~\eqref{eq:obj_subgrad_cond}.} Since $V_{t+1}$ spans $v$, there exists a vector $s \in \RR^k$ such that $V_{t+1}s = v$. Taking $\eta = 0$ and $S = \alpha ss^{\!\top}$ implies $\alpha vv^{\!\top} \in \widehat{\cX}_{t+1}$. Hence, 
\begin{equation*}
    \begin{aligned}
    \hat{f}_{t+1}(y) &\geq \langle C - \cA\adj y, \alpha v v^{\!\top} \rangle + \langle b, y \rangle \\
    &= \langle C - \cA\adj, \alpha v v^{\!\top} \rangle + \langle b, \tilde{y}_{t+1} \rangle + \langle b + \alpha \cA (v v^{\!\top}), y - \tilde{y}_{t+1}\rangle \\
    &= f(\tilde{y}_{t+1}) + \langle g_{t+1}, y - \tilde{y}_{t+1} \rangle.
    \end{aligned}
\end{equation*}

\paragraph{Verifying~\eqref{eq:model_subgrad_cond}.} From the first-order optimality conditions and the update step~\eqref{eq:dual_update} we know that
\begin{equation*}
\begin{aligned}
    s_{t+1} &= \rho(y_t - \tilde{y}_{t+1}) = b - \nu_{t+1} - \cA X_{t+1},  \\
    \hat{f}_t(\tilde{y}_{t+1}) &= \langle C - \cA\adj \tilde{y}_{t+1}, X_{t+1} \rangle + \langle b - \nu_{t+1}, \tilde{y}_{t+1} \rangle.
\end{aligned}
\end{equation*}
To show the desired result, we first want to show that $X_{t+1} \in \widehat{X}_{t+1}$. If $k_p = 0$, we are done since $X_{t+1} = \bar{X}_{t+1}$.
Otherwise, $k_p \geq 1$. First note that $\tr(X_{t+1}) \leq \alpha$ by construction.
Then,
\begin{align*}
    X_{t+1} 
    &= \eta_{t+1} \bar{X}_t + V_t S_{t+1} V_t^\top \\
    &= \eta_{t+1} \bar{X}_t + V_t (Q_{\overline{p}} \Lambda_{\overline{p}}  Q_{\overline{p}}^\top + Q_{\underline{c}} \Lambda_{\underline{c}}  Q_{\underline{c}}^\top) V_t^\top \\
    &= \eta_{t+1} \bar{X}_t + V_t Q_{\overline{p}} \Lambda_{\overline{p}}  Q_{\overline{p}}^\top V_t^\top + V_t Q_{\underline{c}} \Lambda_{\underline{c}}  Q_{\underline{c}}^\top V_t^\top \\
    &= \bar{X}_{t+1} +  V_t Q_{\overline{p}} \Lambda_{\overline{p}}  Q_{\overline{p}}^\top V_t^\top.
\end{align*}
Since $V_{t+1}$ spans each of the columns of $V_t Q_{\overline{p}}$, we can conclude that $X_{t+1} \in \widehat{X}_{t+1}$. Thus, for any $y \in \cY$,
\begin{equation*}
    \hat{f}_{t+1}(y) \geq \langle C - \cA\adj y, X_{t+1} \rangle + \langle b - \nu_{t+1}, y \rangle = \hat{f}_t (\tilde{y}_{t+1}) + \langle s_{t+1}, y - \tilde{y}_{t+1}\rangle.
\end{equation*}
